# Supplementary material for: Time series models for realized covariance matrices based on the matrix-F distribution
Source: arXiv:1903.12077 ancillary file (2020-07-09)
Supplement: Supplementary file 1 [file Supplementary_material.pdf]

# SUPPLEMENT TO "TIME SERIES MODELS FOR REALIZED COVARIANCE MATRICES BASED ON THE MATRIX-F DISTRIBUTION"

By Jiayuan Zhou*, Feiyu Jiang[†], Ke Zhu[‡] and Wai Keung Li[‡§]

*University of Florida*, Tsinghua University,*[†]

*The University of Hong Kong*[‡] *and The Education University of Hong Kong*[§]

This supplement provides four appendices for the paper. Appendix A gives the proofs of Theorem 2.1. Appendix B gives the proofs for Theorems 3.1-5.6. Appendix C provides the proofs of lemmas used in Appendices A and B. Appendix D lists some useful derivatives.

## APPENDIX A: PROOF OF THEOREM 2.1.

This appendix contains the proof of Theorem 2.1. To facilitate the proof, we recall some results in Boussama et al. (2011).

Theorem A.1. *Let there be a multivariate semi-polynomial Markov Chain, which is of the form $X_{t+1} = \mathcal{E}(X_t, \delta_t)$ , where $X_t$ is of dimension $m_1$, $\delta_t$ is i.i.d. sequence of dimension $m_2$, and $\mathcal{E}$ is a $\mathcal{C}^1$ continuous map. Let $V \subseteq \mathbb{R}^{m_1}$ be an algebraic variety and $U$ be an open subset of $\mathbb{R}^{m_1}$.*

*Suppose there exist $\mathcal{C}^1$ continuous maps $\mathcal{L}$ and $\upsilon$ to satisfy the decomposition $\mathcal{E}(z, y) = \mathcal{L}(z, \upsilon(z, y))$ and the regularity conditions in Section 3 of Boussama et al. (2011) hold.*

*Then if the following assumptions (S1)-(S4) hold, there exists a unique strict stationary solution to $X_t$ which is Harris-recurrent and geometrically $\beta$-mixing.*

*(S1) $\delta_t$ is i.i.d. with distribution $\Gamma$ which is absolutely continuous with respect to Lebesgue measure on $\mathbb{R}^{m_2}$.*

*(S2) Define for all $k \in \mathbb{N}^*\backslash\{1\}$, the function $\mathcal{E}^k(z, \delta_1, \ldots, \delta_k) := \mathcal{E}(\mathcal{E}^{k-1}(z, \delta_1, \ldots, \delta_{k-1}), \delta_k)$ for $z \in U$, $\delta_1, \ldots, \delta_k \in \mathbb{R}^{m_1}$. Then for any $z \in V \cap U$ we can define an orbit:*

$$S_z := \bigcup_{k\in\mathbb{N}^*} \left\{\mathcal{E}^k(z, y_1, \ldots, y_k) : \; y_1, \ldots, y_k \in E\right\} = \bigcup_{k\in\mathbb{N}^*} \mathcal{E}^k(z, E^k),$$

*where $E$ denotes the support of $\Gamma$. There exist a point $a_0 \in int(E)$ and a point $\Lambda \in W \bigcap U$, where $W := \overline{^Z S_\Lambda}$ as the Zariski closure of the orbit $S_\Lambda$, such that for all*

*$z \in W \bigcap U$ the sequence $\{X_t^z : X_t^z = F(X_{t-1}^z, a_0), X_0^z = z\}$ converges to the point $\Lambda$.*

*(S3) The strict stationary solution of the Markov chain $X_t = \mathcal{E}(X_{t-1}, \delta_t)$ takes its values in the algebraic variety $W \bigcap U$.*

*(S4) The Forster-Lyapunov (FL) condition hold, i.e., there exist a function $V : U \to [1, \infty]$ and positive constants $\alpha < 1$, $b < \infty$ as well as a Borel set $\mathcal{K}$ in $W \cap U$ such that the (FL) condition hold, i.e.*

$$PV(x) \leq \alpha V(x) + b \cdot 1_K(x), \quad \forall x \in W \bigcap U.$$

Proof of Theorem 2.1. Applying $vec(\cdot)$ operation to both sides of model (2.3), we have $\sigma_t = \wr + \sum_{i=1}^{M} (A_i^* y_{t-i} + B_i^* \sigma_{t-i})$, where $\sigma_t = vec(\Sigma_t)$, $y_t = vec(Y_t)$, and $\wr = vec(\Omega)$. Define process $X_t$ as

$$X_t = \begin{pmatrix} \sigma_t \\ \vdots \\ \sigma_{t-M+1} \\ y_t \\ \vdots \\ y_{t-M+1} \end{pmatrix} = \begin{pmatrix} \wr + \sum_{i=1}^{M} (A_i^* y_{t-i} + B_i^* \sigma_{t-i}) \\ \vdots \\ \sigma_{t-M+1} \\ y_t \\ \vdots \\ y_{t-M+1} \end{pmatrix}. \tag{A.1}$$

Then, by (S1)-(S4), there exist some maps $\mathcal{E}$, $\mathcal{L}$ and $\upsilon$ such that

$$X_t = \mathcal{E}(X_{t-1}, \delta_t) = \mathcal{L}(X_{t-1}, y_t) = \mathcal{L}(X_{t-1}, \upsilon(X_{t-1}, \delta_t)),$$

where $y_t = \upsilon(X_{t-1}, \delta_t)$ and $\delta_t = vec(\Delta_t)$. Since $\mathcal{E},\ \mathcal{L},\ \upsilon$ are $\mathcal{C}^1$ continuous by lemma 4.1 of Boussama et al. (2011), it is obvious that the CBF model has stationary solution if and only if (A.1) has stationary solution, which is the case by (S1)-(S4) according to Theorem A.1. Hence, the proof is completed if (S1)-(S4) hold. Notice (S1) automatically holds by (H1). Then, it suffices to check (S2)-(S4) by Lemmas A.1-A.3 below, respectively. □

Lemma A.1. *Suppose that (H1)-(H3) hold. For the constructed markov chain $Z_t$, (S2) holds by choosing $a_0 = vec(I_n)$ and $\Lambda$ defined via the following equation: $\Lambda = (\wr', 0, \ldots, 0)' +$*

$\Psi\Lambda$, *where* $\Psi = \begin{pmatrix} \mathcal{B}+\mathcal{A} & 0 \\ 0 & \mathcal{B}+\mathcal{A} \end{pmatrix} \in \mathbb{R}^{2Mn^2\times 2Mn^2}$ *with*

$$\mathcal{A} = \begin{pmatrix} A_1^* & A_2^* & \ldots & A_{M-1}^* & A_M^* \\ 0 & 0 & \cdots & 0 & 0 \\ 0 & \ddots & \ddots & \vdots & \vdots \\ \vdots & \ddots & 0 & 0 & 0 \\ 0 & \cdots & 0 & 0 & 0 \end{pmatrix} \in \mathcal{R}^{Mn^2\times Mn^2},$$

$$\mathcal{B} = \begin{pmatrix} B_1^* & B_2^* & \ldots & B_{M-1}^* & B_M^* \\ I_{n^2} & 0 & \cdots & 0 & 0 \\ 0 & \ddots & \ddots & \vdots & \vdots \\ \vdots & \ddots & I_{n^2} & 0 & 0 \\ 0 & \cdots & 0 & I_{n^2} & 0 \end{pmatrix} \in \mathcal{R}^{Mn^2\times Mn^2}.$$

LEMMA A.2. *Suppose that (H1)-(H3) hold. Then, (S3) holds, i.e., the strict stationary solution of* $X_t$ *takes value in* $W \cap U$.

LEMMA A.3. *Suppose that (H1)-(H3) hold. Then, the (FL) condition in (S4) holds.*

The proofs of Lemmas A.1-A.3 can be found in the Appendix C.

## APPENDIX B: PROOFS OF THEOREMS 3.1-5.6.

In this appendix, we only give the proofs of Theorems 5.1-5.6. The proofs of Theorems 3.1-3.2 and 4.1 are essentially similar and less complicated, and hence they are omitted. To facilitate the proofs, we define

$$\begin{aligned}
\mathcal{Y}_t &= \big(vec(Y_t)', \cdots, vec(Y_{t-M})'\big)' \in \mathcal{R}^{Mn^2\times 1},\\
\mathcal{H}_t(\delta) &= \big(vec(\Sigma_{vt}(\delta))', \cdots, vec(\Sigma_{vt-M}(\delta))'\big)' \in \mathcal{R}^{Mn^2\times 1},\\
\widehat{\mathcal{H}}_t(\delta) &= \big(vec(\widehat{\Sigma}_{vt}(\delta))', \cdots, vec(\widehat{\Sigma}_{vt-M}(\delta))'\big)' \in \mathcal{R}^{Mn^2\times 1},\\
r(\delta) &= \left(s'\left[I_{n^2} - \sum_{i=1}^{M}(A_i^* + B_i^*)\right]', 0_{1\times(M-1)n^2}\right)' \in \mathcal{R}^{Mn^2\times 1}.
\end{aligned}$$

Then, the recursion (5.5) can be rewritten as

$$\widehat{\mathcal{H}}_t(\delta) = r(\delta) + \mathcal{A}(u)\mathcal{Y}_{t-1} + \mathcal{B}(u)\widehat{\mathcal{H}}_{t-1}(\delta), \tag{B.1}$$

where $\mathcal{A}$ and $\mathcal{B}$ defined as in Lemma A.1 are functions of $u$, $\mathcal{Y}_0 = \mathcal{Y}_0^*$ and $\widehat{\mathcal{H}}_0(\delta) = \widehat{\mathcal{H}}_0^*$ are calculated based on the sequence of given initial constant matrices $h$. Similarly, the recursion (5.7) can be rewritten as

$$\mathcal{H}_t(\delta) = r(\delta) + \mathcal{A}(u)\mathcal{Y}_{t-1} + \mathcal{B}(u)\mathcal{H}_{t-1}(\delta). \tag{B.2}$$

It is worth noting that when $E\|Y_t\| < \infty$, by Theorem 2.1 and a similar argument as for (B.15) in Pedersen and Rahbek (2014), there exists $0 < \phi < 1$, such that for any integer $i \geq 0$,

$$\sup_{u\in\Theta_u} \|\mathcal{B}^i(u)\| \leq U\phi^i, \tag{B.3}$$

where $U > 0$ is a generic constant in the sequel.

Moreover, we give five technical lemmas. Lemma B.1 provides a list of useful results in matrix algebra. Lemma B.2 presents some moment conditions related to $\Sigma_t(\delta)$. Lemma B.3 ensures that the effect of the first-step estimation and the initial values is negligible for the second-step estimation. Lemma B.4 is standard to prove the strong consistency of $\widehat{\theta}_v$. Lemma B.5 is needed for the identifiability of $\widehat{\theta}_v$. The proofs of Lemmas B.1-B.5 can be found in the Appendix C.

LEMMA B.1. *Suppose that $A$, $B$, $C$ and $D$ are $n \times n$ square matrices. Then,*

(i) $tr(ABCD) = vec(D')'(C' \otimes A)vec(B) = (vec(D))'(A \otimes C')vec(B')$;

(ii) $tr(A \otimes B) = tr(A)tr(B)$;

(iii) $\|tr(AB)\| \leq \|A\|\,\|B\|$;

(iv) $\|A\|_{spec} \leq \|A\| \leq \sqrt{n}\,\|A\|_{spec}$;

(v) $\|AB\| \leq \|A\|_{spec}\|B\|$ *and* $\|A+B\|_{spec} \leq \|A\|_{spec} + \|B\|_{spec}$;

(vi) *For* $A > 0$, $\|A\| \leq tr(A)$ *and* $\left\|(I+A)^{-1}\right\| \leq \sqrt{n}$;

(vii) *For* $A > 0$, $\log|A| \leq tr(A)$, $\log|A| \leq n\log\|A\|_{spec}$, *and* $\|\log|A|\| \leq tr(A) + tr(A^{-1})$;

(viii) *For* $A > 0$, $|A+B| \geq |B|$;

(ix) *For* $A \geq 0$ *and* $B > 0$, $0 < tr\left[(A+B)^{-1}\right] \leq tr(B^{-1})$;

(x) *For* $A > 0$ *and* $B > 0$, $\left\|\log|AB^{-1}|\right\| \leq n\|A-B\|\left(\|B^{-1}\| + \|A^{-1}\|\right)$.

LEMMA B.2. *Let $\delta_i$ be the $i$-th entry of $\delta$. Suppose that Assumption 3.1 holds. Then,*

(i) $\sup_{\delta\in\Theta_\delta} \|\Sigma_{vt}^{-1}(\delta)\| \leq U$;

(ii) $\sup_{\delta\in\Theta_\delta} \|\widehat{\Sigma}_{vt}^{-1}(\delta)\| \leq U$;

(iii) *If* $E\|Y_t\|^k < \infty$, $E\left[\left(\sup_{\delta\in\Theta_\delta}\|\Sigma_{vt}(\delta)\|\right)^k\right] < \infty$ *for some* $k \geq 1$;

(iv) *If* $E\|Y_t\|^k < \infty$, $E\left[\left(\sup_{\delta\in\Theta_\delta}\left\|\frac{\partial\Sigma_{vt}(\delta)}{\partial\delta_i}\right\|\right)^k\right] < \infty$ *for some* $k \geq 1$ *and each* $i = 1, 2, \cdots, \tau_2$;

(v) *If* $E\|Y_t\|^k < \infty$, $E\left[\left(\sup_{\delta\in\Theta_\delta}\left\|\frac{\partial^2\Sigma_{vt}(\delta)}{\partial\delta_i\partial\delta_j}\right\|\right)^k\right] < \infty$ *for some* $k \geq 1$ *and each* $i, j = 1, 2, \cdots, \tau_2$.

Lemma B.3. *Suppose that Assumptions 3.1 and 3.2 hold and* $E\|Y_t\| < \infty$. *Then,*

$$\sup_{(u,\nu)\in\Theta_u\times\Theta_\nu}\left\|L_v(s_0, u, \nu) - \widehat{L}_v(\widehat{s}_v, u, \nu)\right\| \xrightarrow{a.s.} 0 \quad \text{as } T \to \infty.$$

Lemma B.4. *Suppose that Assumptions 3.1 and 3.2 hold and* $E\|Y_t\| < \infty$. *Then,*

(i) $E\left[\sup_{\theta_v\in\Theta_v}\|l_{vt}(\theta_v)\|\right] < \infty$;

(ii) $\sup_{\theta_v\in\Theta_v}\|L_v(\theta_v) - E[l_{vt}(\theta_v)]\| \xrightarrow{a.s.} 0$ *as* $T \to \infty$.

Lemma B.5. *For any* $(u_0, \nu_0) \neq (u, \nu)$, $E[l_{vt}(s_0, u_0, \nu_0)] < E[l_{vt}(s_0, u, \nu)]$.

Proof of Theorem 5.1. First, by the ergodic theorem, we have

$$\widehat{s}_v \xrightarrow{a.s} s_0 \quad \text{as } T \to \infty.$$

Second, we can show that when $T$ is large, for any $\varepsilon > 0$,

$$\begin{aligned}
&E[l_{vt}(s_0, \widehat{u}_v, \widehat{\nu}_v)] < L_v(s_0, \widehat{u}_v, \widehat{\nu}_v) + \frac{\varepsilon}{5} \quad \text{by Lemma B.4(ii);}\\
&L_v(s_0, \widehat{u}_v, \widehat{\nu}_v) < \widehat{L}_v(\widehat{s}_v, \widehat{u}_v, \widehat{\nu}_v) + \frac{\varepsilon}{5} \quad \text{by Lemma B.3;}\\
&\widehat{L}_v(\widehat{s}_v, \widehat{u}_v, \widehat{\nu}_v) < \widehat{L}_v(\widehat{s}_v, u_0, \nu_0) + \frac{\varepsilon}{5} \quad \text{by definition of } \widehat{\mu}_v, \widehat{\nu}_v;\\
&\widehat{L}_v(\widehat{s}_v, u_0, \nu_0) < L_v(s_0, u_0, \nu_0) + \frac{\varepsilon}{5} \quad \text{by Lemma B.2;}\\
&L_v(s_0, u_0, \nu_0) < E[l_{vt}(s_0, u_0, \nu_0)] + \frac{\varepsilon}{5} \quad \text{by Lemma B.4(ii).}
\end{aligned}$$

Thus, when $T$ is large, for any $\varepsilon > 0$, $E[l_{vt}(s_0, \widehat{u}_v, \widehat{\nu}_v)] < E[l_{vt}(s_0, u_0, \nu_0)] + \varepsilon$. By Lemma B.5 and the continuity of the log-likelihood function, it follows that $(\widehat{u}_v, \widehat{\nu}_v) \xrightarrow{a.s.} (u_0, \nu_0)$ by Theorem 2.1 in Newey and McFadden (1994). This completes the proof. □

In order to prove Theorem 5.2, we need four more lemmas. Lemmas B.6-B.8 present some standard technical conditions, and Lemma B.9 ensures the negligibility of the initial values. The proofs of Lemmas B.6-B.9 can be found in the supplementary material.

LEMMA B.6. *Let $\theta_{vi}$ be the $i$-th entry of $\theta_v$. Suppose that Assumptions 3.1 and 3.2 hold and $E\|Y_t\|^2 < \infty$. Then,*
(i) $E\left[\sup_{\theta_v \in \Theta_v} \left\| \frac{\partial^2 l_{vt}(\theta_v)}{\partial\theta_{vi}\partial\theta_{vj}} \right\|\right] < \infty$;
(ii) $\sup_{\theta_v \in \Theta_v} \left\| \frac{\partial^2 L_v(\theta_v)}{\partial\theta_{vi}\partial\theta_{vj}} - E\left[\frac{\partial^2 l_{vt}(\theta_v)}{\partial\theta_{vi}\partial\theta_{vj}}\right] \right\| \xrightarrow{a.s} 0$ *as* $T \to \infty$,
*for each* $i, j = 1, 2, \cdots, \tau_2$.

LEMMA B.7. *Suppose that Assumptions 3.1 and 3.2 hold and $E\|Y_t\|^2 < \infty$. Then,*

$$\sqrt{T}\begin{pmatrix} \widehat{s}_v - s_0 \\ \partial L_v(\theta_{v0})/\partial\zeta \end{pmatrix} = \frac{1}{\sqrt{T}}\sum_{t=1}^{T} w_t + o_p(1),$$

*where $w_t$ is defined as in Theorem 5.2 and $E(w_t|\mathcal{G}_{t-1}) = 0$.*

LEMMA B.8. *Suppose that Assumptions 3.1 and 3.2 hold and $E\|Y_t\|^2 < \infty$. Then,*

$$\frac{1}{\sqrt{T}}\sum_{t=1}^{T} w_t \xrightarrow{d} N(0, E\left[w_t w_t'\right]) \quad \text{as } T \to \infty.$$

LEMMA B.9. *Suppose that Assumptions 3.1 and 3.2 hold and $E\|Y_t\|^3 < \infty$. Then,*
(i) $\sup_{\theta_v \in \Theta_v} \left\| \sqrt{T}\left(\frac{\partial L_v(\theta_v)}{\partial\theta_{vi}} - \frac{\partial \widehat{L}_v(\theta_v)}{\partial\theta_{vi}}\right) \right\| \xrightarrow{p} 0$ *as* $T \to \infty$;
(ii) $\sup_{\theta_v \in \Theta_v} \left\| \frac{\partial^2 L_v(\theta_v)}{\partial\theta_{vi}\partial\theta_{vj}} - \frac{\partial^2 \widehat{L}_v(\theta_v)}{\partial\theta_{vi}\partial\theta_{vj}} \right\| \xrightarrow{p} 0$ *as* $T \to \infty$,
*for each $i, j = 1, 2, \cdots, \tau_2$, where $\theta_{vi}$ is the $i$-th entry of $\theta_v$.*

PROOF OF THEOREM 5.2. By the mean value theorem, there exist $\theta_*$ between $\theta_{v0}$ and $\widehat{\theta}_v$ such that $0 = \frac{\partial \widehat{L}_v(\theta_{v0})}{\partial\zeta} + \frac{\partial^2 \widehat{L}_v(\theta_*)}{\partial\zeta\partial s'}(\widehat{s}_v - s_0) + \frac{\partial^2 \widehat{L}_v(\theta_*)}{\partial\zeta\partial\zeta'}(\widehat{\zeta}_v - \zeta_0)$. Then, by Lemma B.9, we have

$$\begin{aligned} 0 = {} & \sqrt{T}\frac{\partial L_v(\theta_{v0})}{\partial\zeta} + [J_{2T}^* + o_p(1)]\left[\sqrt{T}\left(\widehat{s}_v - s_0\right)\right] \\ & + [J_{1T}^* + o_p(1)]\left[\sqrt{T}\left(\widehat{\zeta}_v - \zeta_0\right)\right] + o_p(1), \end{aligned} \tag{B.4}$$

where $J_{1T}^* = \frac{\partial^2 L_v(\theta_*)}{\partial\zeta\partial\zeta'}$ and $J_{2T}^* = \frac{\partial^2 L_v(\theta_*)}{\partial\zeta\partial s'}$. By Lemma B.6 and Theorem 3.1 in Ling and McAleer (2003), we have $J_{1T}^* = J_1 + o_p(1)$ and $J_{2T}^* = J_2 + o_p(1)$. Hence, by (B.4) and Lemma B.7, it follows that

$$\sqrt{T}(\widehat{\theta}_v - \theta_{v0}) = \begin{pmatrix} I_{n^2} & 0 \\ -J_1^{-1}J_2 & -J_1^{-1} \end{pmatrix}\sqrt{T}\begin{pmatrix} \widehat{s}_v - s_0 \\ \frac{\partial L_v(\theta_{v0})}{\partial\zeta} \end{pmatrix} + o_p(1). \tag{B.5}$$

Finally, the proof is completed by Slutzky's theorem and Lemma B.8. □

Proof of Theorem 5.3. By Taylor's expansion and Theorem 5.2, we can show that

$$\sqrt{T}\mathcal{V}_{vl}(\widehat{\delta}_v) = \frac{1}{\sqrt{T}}\sum_{t=l+1}^{T}\begin{pmatrix}\mathbf{b}_{vt,1}(\delta_0)\\ \mathbf{b}_{vt,2}(\delta_0)\\ \vdots\\ \mathbf{b}_{vt,l}(\delta_0)\end{pmatrix} + \frac{1}{T}\sum_{t=l+1}^{T}\begin{pmatrix}\mathfrak{Z}'_{vt-1}(\delta_0)\left(\partial\mathfrak{Z}_{vt}(\delta_0)/\partial\theta'\right)\\ \mathfrak{Z}'_{vt-2}(\delta_0)\left(\partial\mathfrak{Z}_{vt}(\delta_0)/\partial\theta'\right)\\ \vdots\\ \mathfrak{Z}'_{vt-l}(\delta_0)\left(\partial\mathfrak{Z}_{vt}(\delta_0)/\partial\theta'\right)\end{pmatrix}$$

$$\times\frac{1}{\sqrt{T}}\begin{pmatrix} I_{n^2} & 0\\ -J_1^{-1}J_2 & -J_1^{-1}\end{pmatrix}\sum_{t=1}^{T} w_t(\delta_0) + o_p(1)$$

$$= (I_l, \mathfrak{R}_v)\frac{1}{\sqrt{T}}\sum_{t=l+1}^{T}\mathbf{e}_{vt} + o_p(1).$$

Since $\mathbf{e}_{vt}$ is a martingale difference sequence, the proof follows by standard arguments. □

Next, we consider the proofs of Theorems 5.4 and 5.6. Since the proof of Theorem 5.5 is essentially similar as the one for Theorem 5.6, it is omitted for simplicity.

Proof of Theorem 5.4. Based on Assumptions 5.1-5.3, the proof is the same as the one for Theorem 1 in Shen et al. (2018), hence it is omitted here. □

Proof of Theorem 5.6. First, it is straightforward to show that (i) holds by Theorem 5.4(ii). Next, we can claim that

$$\sup_{\zeta\in\Theta_u\times\Theta_\nu}\left\|\frac{\partial\widehat{L}_{fv}(\widehat{s}_{1fv},\zeta)}{\partial\zeta} - \frac{\partial L_{fv}(\widehat{s}_{2fv},\zeta)}{\partial\zeta}\right\|$$

$$= O_p(B(T)/T) + O_p(A^{1/2}(n,m,T)B^{5/2}(T)). \tag{B.6}$$

In order to prove (B.6), we define

$$\mathcal{Y}_{ft} = \left(vec(Y_{ft})', \cdots, vec(Y_{ft-M})'\right)' \in \mathcal{R}^{Mn^2\times 1},$$

$$\widehat{\mathcal{Y}}_{ft} = \left(vec(\widehat{Y}_{ft})', \cdots, vec(\widehat{Y}_{ft-M})'\right)' \in \mathcal{R}^{Mn^2\times 1},$$

$$\mathcal{H}_{ft}(\delta) = \left(vec(\Sigma_{fvt}(\delta))', \cdots, vec(\Sigma_{fvt-M}(\delta))'\right)' \in \mathcal{R}^{Mn^2\times 1},$$

$$\widehat{\mathcal{H}}_{ft}(\delta) = \left(vec(\widehat{\Sigma}_{fvt}(\delta))', \cdots, vec(\widehat{\Sigma}_{fvt-M}(\delta))'\right)' \in \mathcal{R}^{Mn^2\times 1}.$$

Then, as for (B.1)-(B.2), we have $\widehat{\mathcal{H}}_{ft}(\widehat{s}_{1fv},\zeta) - \mathcal{H}_{ft}(\widehat{s}_{2fv},\zeta) = \left[r(\widehat{s}_{1fv},\zeta) - r(\widehat{s}_{2fv},\zeta)\right] + \mathcal{A}(u)\left[\widehat{\mathcal{Y}}_{ft} - \mathcal{Y}_{ft}\right] + \mathcal{B}(u)\left[\widehat{\mathcal{H}}_{ft-1}(\widehat{s}_{1fv},\zeta) - \mathcal{H}_{ft-1}(\widehat{s}_{2fv},\zeta)\right]$, and since $\rho(\sum_{i=1}^{M} B_i^*) < 1$, it implies that

$$\widehat{\mathcal{H}}_{ft}(\widehat{s}_{1fv},\zeta) - \mathcal{H}_{ft}(\widehat{s}_{2fv},\zeta)$$

$$
\begin{aligned}
&= \mathcal{B}^t(u)(\widehat{\mathcal{H}}_{f0} - \mathcal{H}_{f0}(\widehat{s}_{2fv}, \zeta)) \\
&\quad + \sum_{i=0}^{t-1} \mathcal{B}^i(u) \left\{ [r(\widehat{s}_{1fv}, \zeta) - r(\widehat{s}_{2fv}, \zeta)] + \mathcal{A}(u) \left[ \widehat{\mathcal{Y}}_{ft} - \mathcal{Y}_{ft} \right] \right\} \\
&= \mathcal{B}^t(u)(\widehat{\mathcal{H}}_{f0} - \mathcal{H}_{f0}(s_0, \zeta)) - \mathcal{B}^t(u)(\mathcal{H}_{f0}(\widehat{s}_{2fv}, \zeta) - \mathcal{H}_{f0}(s_0, \zeta)) \\
&\quad + \sum_{i=0}^{t-1} \mathcal{B}^i(u) \left\{ [r(\widehat{s}_{1fv}, \zeta) - r(\widehat{s}_{2fv}, \zeta)] + \mathcal{A}(u) \left[ \widehat{\mathcal{Y}}_{ft} - \mathcal{Y}_{ft} \right] \right\}, \qquad \text{(B.7)}
\end{aligned}
$$

where $\widehat{\mathcal{H}}_{f0}$ is a given initial value. By (B.7), we can show that

$$
\begin{aligned}
&\sup_{\zeta \in \Theta_u \times \Theta_\nu} \left\| \widehat{\Sigma}_{fvt}(\widehat{s}_{1fv}, \zeta) - \Sigma_{fvt}(\widehat{s}_{2fv}, \zeta) \right\| \\
&= O_p(\phi^t) + O_p(\phi^t/\sqrt{T}) + O_p(A^{1/2}(n, m, T) B^{3/2}(T)), \qquad \text{(B.8)} \\
&\sup_{\zeta \in \Theta_u \times \Theta_\nu} \left\| \widehat{\Sigma}_{fvt}^{-1}(\widehat{s}_{1fv}, \zeta) \widehat{Y}_{ft} - \Sigma_{fvt}^{-1}(\widehat{s}_{2fv}, \zeta) Y_{ft} \right\| \\
&= \sup_{\zeta \in \Theta_u \times \Theta_\nu} \Big\| \widehat{\Sigma}_{fvt}^{-1}(\widehat{s}_{1fv}, \zeta)(\widehat{Y}_{ft} - Y_{ft}) \\
&\quad - \Sigma_{fvt}^{-1}(\widehat{s}_{2fv}, \zeta) \left[ \Sigma_{fvt}(\widehat{s}_{2fv}, \zeta) - \widehat{\Sigma}_{fvt}(\widehat{s}_{2fv}, \zeta) \right] \widehat{\Sigma}_{fvt}^{-1}(\widehat{s}_{1fv}, \zeta) Y_{ft} \Big\| \\
&= \left[ O_p(\phi^t) + O_p(\phi^t/\sqrt{T}) + O_p(A^{1/2}(n, m, T) B^{3/2}(T)) \right] [1 + O_p(B(T))], \qquad \text{(B.9)}
\end{aligned}
$$

where (B.8) holds by (B.3), the compactness of $\Theta_u$ and $\Theta_\nu$, Lemma B.2(iii)-(iv) and Theorems 5.1 and 5.4, and (B.9) holds by the triangular inequality, Lemma B.2(i)-(ii), (B.8), and Assumption 5.2.

Now, by (B.8)-(B.9) and Lemma B.1(x), we can show that $\sup_{\zeta \in \Theta_u \times \Theta_\nu} \| \frac{\partial \widehat{L}_{fv}(\widehat{s}_{1fv}, \zeta)}{\partial \zeta} - \frac{\partial L_{fv}(\widehat{s}_{2fv}, \zeta)}{\partial \zeta} \| = \sum_{t=1}^T [O_p(\phi^t) + O_p(\phi^t/\sqrt{T}) + O_p(A^{1/2}(n, m, T) B^{3/2}(T))][1 + O_p(B(T))]$, i.e., (B.6) holds. By (B.6) and Taylor's expansion, we have

$$
\begin{aligned}
0 = \frac{\partial \widehat{L}_{fv}(\widehat{s}_{1fv}, \widehat{\zeta}_{1fv})}{\partial \zeta} &= \frac{\partial L_{fv}(\widehat{s}_{2fv}, \widehat{\zeta}_{1fv})}{\partial \zeta} + O_p(B(T)/T) + O_p(A^{1/2}(n, m, T) B^{5/2}(T)) \\
&= \frac{\partial L_{fv}(\widehat{s}_{2fv}, \widehat{\zeta}_{2fv})}{\partial \zeta} + \frac{\partial L_{fv}(\widehat{s}_{2fv}, \widehat{\xi}_{fv})}{\partial \zeta \partial \zeta'} (\widehat{\zeta}_{1fv} - \widehat{\zeta}_{2fv}) \\
&\quad + O_p(B(T)/T) + O_p(A^{1/2}(n, m, T) B^{5/2}(T)) \\
&= \left\{ E \left[ \frac{\partial l_{fvt}(\widehat{s}_{2fv}, \widehat{\xi}_{fv})}{\partial \zeta \partial \zeta'} \right] + o_p(1) \right\} (\widehat{\zeta}_{1fv} - \widehat{\zeta}_{2fv}) \\
&\quad + O_p(B(T)/T) + O_p(A^{1/2}(n, m, T) B^{5/2}(T)),
\end{aligned}
$$

where $\widehat{\xi}_{fv}$ lies between $\widehat{\zeta}_{1fv}$ and $\widehat{\zeta}_{2fv}$, and the fourth equality holds by Lemma B.6 and the law of large numbers theorem for stationary sequence. Hence, by Lemma B.6 again, it follows that (ii) holds. This competes all of the proofs. □

## APPENDIX C: PROOFS OF LEMMAS

PROOF OF LEMMA A.1. Define $W := \overline{{}^{Z}\bigcup_{i\in\mathbb{N}^*}\mathcal{E}^i(\Lambda, vec(S^+_{n\times n})^i)}$, where $vec(S^+_{n\times n})$ denotes the space of vectorized positive definite matrices, and

$$U := \left[vec(S^+_{n\times n})\right]^{(2M)} = \underbrace{vec(S^+_{n\times n}) \times \cdots \times vec(S^+_{n\times n})}_{2M}.$$

For fix any $z \in U$, define $(X^z_n)_{n\in\mathbb{N}^*}$ as $X^z_0 = z$, $X^z_t = \mathcal{E}(X^z_{t-1}, a_0)$ for $t \geq 1$, and correspondingly define $Y^z_t$, $y^z_t$, $\Sigma^z_t$, and $\sigma^z_t$. Since $a_0 = vec(I_n)$, $Y^z_t = \Sigma^z_t$. By the definition of $\Psi$, we have for $t > M$,

$$X^z_t = \left(\wr', 0, \ldots, 0\right)' + \Psi X^z_{t-1}. \tag{C.1}$$

By (H2) and Proposition 4.5 in Boussama et al. (2011), the spectral radius of $\Psi$ is less than 1. Thus, (S2) holds. □

PROOF OF LEMMA A.2. Notice that $X_t = \mathcal{E}(X_{t-1}, \delta_t) = \mathcal{L}(X_{t-1}, y_t)$, where $y_t \in vec(S^+_{n\times n})$, Thus,

$$W = \overline{{}^{Z}\bigcup_{i\in\mathbb{N}^*}\mathcal{E}^i(\Lambda, E^i)} = \overline{{}^{Z}\bigcup_{i\in\mathbb{N}^*}\mathcal{E}^i(\Lambda, vec(S^+_{n\times n})^i)} = \overline{{}^{Z}\bigcup_{i\in\mathbb{N}^*}\mathcal{L}^i(\Lambda, vec(S^+_{n\times n})^i)}.$$

By letting $\mathcal{Y}_t = (y'_t, y'_{t-1}, \ldots, y'_{t-M+1})'$ and $\mathcal{H}_t = (\sigma'_t, \sigma'_{t-1}, \ldots, \sigma'_{t-M+1})'$, we have

$$\begin{aligned} \mathcal{H}_t &= \left(\wr', 0, \ldots, 0\right)' + \mathcal{A}\mathcal{Y}_{t-1} + \mathcal{B}\mathcal{H}_{t-1} \\ &= \left(\wr', 0, \ldots, 0\right)' + (\mathcal{A}+\mathcal{B})\mathcal{H}_{t-1} + \mathcal{A}\mathcal{D}_{t-1}, \end{aligned} \tag{C.2}$$

where $D_t = \mathcal{Y}_t - \mathcal{H}_t$.

Since $\Lambda$ is the fixed point satisfying equation (C.1), it is easy to verify that $\Lambda$ is unique and has the form $\Lambda = \begin{pmatrix} \widehat{\sigma}', \ldots, \widehat{\sigma}' \end{pmatrix}'_{2Mn^2\times 1}$, where $\widehat{\sigma} = vec(\widehat{\Sigma})$ satisfies that

$$\widehat{\sigma} = vec(\Omega) + \sum_{i=1}^{M}(A^*_i + B^*_i)\widehat{\sigma}. \tag{C.3}$$

By the definition of $W$, $X_0 = \Lambda$, and hence $H_0 = \tilde{\Lambda}$ and $D_0 = 0$, where $\tilde{\Lambda} = \begin{pmatrix} \widehat{\sigma}', \ldots, \widehat{\sigma}' \end{pmatrix}'_{Mn^2\times 1}$. Then, from (C.2) we have

$$\mathcal{H}_t = \underbrace{\sum_{i=0}^{t-1}(\mathcal{A}+\mathcal{B})^i \left(\wr', 0, \ldots, 0\right)' + (\mathcal{A}+\mathcal{B})^t\widehat{\Lambda}}_{=\widehat{\Lambda}} + \sum_{i=1}^{t}(\mathcal{A}+\mathcal{B})^{i-1}\mathcal{A}\mathcal{D}_{t-i}$$

$$= \tilde{\Lambda} + \sum_{i=1}^{t-1} (\mathcal{A}+\mathcal{B})^{i-1}\mathcal{A}\mathcal{D}_{t-i}. \tag{C.4}$$

Let $d_t = y_t - \sigma_t$. It is not hard to see that for $i = 1, 2, \cdots, t-1$, $(\mathcal{A}+\mathcal{B})^{i-1}\mathcal{A}D_{t-i} = \sum_{j=1}^{M}[(\mathcal{A}+\mathcal{B})^{i-1}\mathcal{A}]_{1,j}d_{t-j}$, where $[\cdot]_{1,j}$ represent the $n^2 \times n^2$ block obtained from rows $1 : n^2$ and columns $(j-1)n^2 : jn^2$ of the matrix. By (C.4), it follows that

$$\sigma_t = \widehat{\sigma} + \sum_{i=1}^{t-1} K_i d_{t-i} \tag{C.5}$$

with $K_i = \sum_{j=1}^{M}\left[(\mathcal{A}+\mathcal{B})^{i-j}\mathcal{A}\right]_{1,j}$, where we have used the convention that $A^0 = I$ and $A^i = 0$ if $i < 0$. Thus, we can conclude that $W$ equals the Zariski closure of the orbit

$$\begin{aligned} S_{\Lambda} &= \bigcup_{n\in\mathbb{N}^*} \left\{X_t : y_1, \ldots, y_t \in vec(S^+_{n\times n})\right\} \\ &= \bigcup_{n\in\mathbb{N}^*} \left\{ (\Lambda'_*, y'_t, ..., y'_{t-M+1})' : y_1, \ldots, y_t \in vec(S^+_{n\times n})\right\}, \end{aligned} \tag{C.6}$$

where $\Lambda_* = \left(\tilde{\Lambda} + \left(\left(\sum_{i=1}^{t-1} K_i d_{t-i}\right)', \ldots, \left(\sum_{i=1}^{t-M} K_i d_{t-M+1-i}\right)'\right)'\right)'$.

Now, we suppose $X(t)$ is a strict stationary solution to the process $X_t$, and define $\mathcal{Y}(t)$, $\mathcal{H}(t)$, $\mathcal{D}(t)$, $Y(t)$, $\Sigma(t)$, $y(t)$ and $\sigma(t)$ correspondingly. Then,

$$\begin{aligned} \mathcal{H}(t) &= (\imath', 0, \ldots, 0)' + \mathcal{A}\mathcal{Y}(t-1) + \mathcal{B}\mathcal{H}(t-1) \\ &= (\imath', 0, \ldots, 0)' + (\mathcal{A}+B)\,\mathcal{H}(t-1) + \mathcal{A}\mathcal{D}(t-1) \\ &= \lim_{k\to\infty}\left\{\sum_{i=0}^{k} (\mathcal{A}+\mathcal{B})^i (\imath', 0, \ldots, 0)' + \sum_{i=1}^{k+1} (\mathcal{A}+\mathcal{B})^{i-1}\mathcal{A}\mathcal{D}(t-i) \right. \\ &\qquad \left. + (\mathcal{A}+\mathcal{B})^{k+1}\mathcal{H}(t-k-1)\right\} \\ &= \tilde{\Lambda} + \sum_{i=1}^{\infty} (\mathcal{A}+\mathcal{B})^{i-1}\mathcal{A}\mathcal{D}(t-i) \text{ a.s.,} \end{aligned} \tag{C.7}$$

where the last equation holds by (H3), the stationarity of $\mathcal{H}(t-k)$, and the facts that $(\mathcal{A}+\mathcal{B})^k\mathcal{H}(t-k) \to 0$ a.s. as $k \to \infty$ and

$$\begin{aligned} \sum_{i=0}^{\infty} (\mathcal{A}+\mathcal{B})^i (\imath', 0, \ldots, 0)' &= (\imath', 0, \ldots, 0)' + \sum_{i=1}^{\infty} (\mathcal{A}+\mathcal{B})^i (\imath', 0, \ldots, 0)' \\ &= (\imath', 0, \ldots, 0)' + (\mathcal{A}+\mathcal{B})\sum_{i=0}^{\infty} (\mathcal{A}+\mathcal{B})^i (\imath', 0, \ldots, 0)', \end{aligned}$$

which implies $\sum_{i=0}^{\infty} (\mathcal{A}+\mathcal{B})^i (\imath', 0, \ldots, 0)' = \widehat{\sigma}$.

Notice that the decomposition of (C.7) gives us that $\sigma(t) = \widehat{\sigma} + \sum_{i=1}^{\infty} K_i d(t)$ a.s. Thus, by (C.5)-(C.6) and the closeness of Zariski closure, the strict stationary solution of $X_t$ takes value in $W \cap U$. This completes the proof.

$\square$

Proof of Lemma A.3. For notation convenience, we consider the case that $K = 1$ in model (2.3), since the extension to larger values of $K$ is essentially the same. Define $V(X_t)$ for any $X_t \in W \bigcap U$ as

$$V(X_t) = tr(V_1\Sigma_t) + \cdots + tr(V_M\Sigma_{t-M+1}) + tr(V_{M+1}Y_t) + \cdots + tr(V_{2M}Y_{t-M+1}) + 1,$$

where

$$V_k = \frac{M-k+1}{2M}\Omega + \sum_{j=k}^{M} B_j'\Sigma B_j \quad \text{and} \quad V_{M+k} = \frac{M-k+1}{2M} + \sum_{i=k}^{M} A_i'\Sigma A_i$$

for $1 \leq k \leq M$, and $\Sigma$ satisfies the following equation $\Sigma = \Omega + \sum_{i=1}^{P} A_i\Sigma A_i' + \sum_{j=1}^{M} B_j\Sigma B_j'$. By Proposition 4.3 of Boussama et al. (2011), the existence of such $\Sigma$ is guaranteed under (H1)-(H3).

By simple calculation, we have

$$\begin{aligned}
&E(V(X_t)|X_{t-1})\\
=&E(tr(V_1\Sigma_t) + tr(V_{M+1}Y_t)|X_{t-1}) + tr(V_2\Sigma_{t-1}) + \cdots + tr(V_M\Sigma_{t-M+1})\\
&+ tr(V_{M+2}Y_{t-1}) + \cdots + tr(V_{2M}Y_{t-M+1}) + 1\\
=&tr[(B_1'(V_1 + V_{M+1})B_1' + V_2)\Sigma_{t-1}] + \cdots + tr[(B_{M-1}'(V_1 + V_{M+1})B_{M-1}' + V_M)\Sigma_{t-M+1}]\\
&+ tr[(A_1'(V_1 + V_{M+1})A_1' + V_{M+2})Y_{t-1}] + \cdots + tr[(A_{M-1}'(V_1 + V_{M+1})A_{M-1}' + V_{2M})Y_{t-M+1}]\\
&+ tr[(B_M'(V_1 + V_{M+1})B_M')\Sigma_{t-M}] + tr[(A_M'(V_1 + V_{M+1})A_M')Y_{t-M}] + tr[(V_1 + V_{M+1})\Omega] + 1.
\end{aligned}$$

By the definition of $V_i$, we can deduce the following facts:

$$\begin{aligned}
B_k'(V_1 + V_{M+1})B_k + V_{k+1} &= V_k - \frac{\Omega}{2M}, \quad 1 \leq k \leq M-1;\\
B_M'(V_1 + V_{M+1})B_M &= V_M - \frac{\Omega}{2M};\\
A_k'(V_1 + V_{M+1})A_k + V_{M+k+1} &= V_{M+k} - \frac{\Omega}{2M}, \quad 1 \leq k \leq M-1;\\
A_k'(V_1 + V_{M+1})A_k &= V_{2M} - \frac{\Omega}{2M}.
\end{aligned}$$

Next, we define

$$\alpha_k := \max\{r'(V_k - \frac{\Omega}{2M})r: \ r \in \mathbb{R}^n, r'V_kr = 1\},$$

which is attainable due to the compactness of the sphere $r'V_k r = 1$, and we consider the corresponding value of $r$ as $r_k$, which gives $0 \le \alpha_k = 1 - r_k' \frac{\Omega}{2M} r_k < 1$.

Furthermore, we define $\alpha_0 = \max\{\alpha_k : 1 \le k \le 2M\}$. Then, $\forall k \in \{1, \dots, 2M\}$, we can show that $V_k - \frac{\Omega}{2M} \le \alpha_0 V_k$. Therefore, for any matrix $\Upsilon \in S^+_{n\times n}$ and for all $k \in \{1, \dots, 2M\}$,

$$tr\left[\left(V_k - \frac{\Omega}{2M}\right)\Upsilon\right] \le \alpha_0 tr\left(V_k \Upsilon\right).$$

Thus, it is able to deduce that $E(V(X_t)|X_{t-1} = x) \le \alpha_0 V(x) + tr\left(\Sigma\Omega\right) + 1 - \alpha_0$. Set $\alpha = (\alpha_0 + 1)/2$ and $b = tr(\Sigma\Omega) + 1 - \alpha_0$. Then, the FL condition is satisfied by defining $K$ as

$$K = \left\{x \in W \bigcap U : V(x) \le \frac{b}{\alpha - \alpha_0}\right\}.$$

The compactness of $K$ can be shown by the similar ideas as in Section 4.6 in Boussama et al. (2011). This completes the proof. □

Proof of Lemma B.1. The proofs of (i)-(ix) can be found in Appendix B of Pedersen and Rahbek (2014), and (x) holds by the fact that

$$\begin{aligned}
\left\|\log\left|AB^{-1}\right|\right\| &= \log\left|AB^{-1}\right| \mathbb{1}\left(|AB^{-1}| \ge 1\right) + \log\left|BA^{-1}\right| \mathbb{1}\left(|BA^{-1}| \ge 1\right) \\
&\le n\log\|AB^{-1}\|_{spec}\mathbb{1}\left(|AB^{-1}| \ge 1\right) + n\log\|BA^{-1}\|_{spec}\mathbb{1}\left(|BA^{-1}| \ge 1\right) \\
&= n\log\|I_n + (A-B)B^{-1}\|_{spec}\mathbb{1}\left(|AB^{-1}| \ge 1\right) \\
&\quad + n\log\|I_n + (B-A)A^{-1}\|_{spec}\mathbb{1}\left(|BA^{-1}| \ge 1\right) \\
&\le n\log\left(1 + \|(A-B)B^{-1}\|_{spec}\right)\mathbb{1}\left(|AB^{-1}| \ge 1\right) \\
&\quad + n\log\left(1 + \|(B-A)A^{-1}\|_{spec}\right)\mathbb{1}\left(|BA^{-1}| \ge 1\right) \\
&\le n\left\{\log\left(1 + \|(A-B)B^{-1}\|\right) + \log\left(1 + \|(B-A)A^{-1}\|\right)\right\} \\
&\le n\left\{\|(A-B)B^{-1}\| + \|(B-A)A^{-1}\|\right\}.
\end{aligned}$$

This completes all of the proofs. □

Proof of Lemma B.2. (i) From (5.1) and (5.7), we have

$$\|\Sigma_{vt}^{-1}(\delta)\| \le tr(\Sigma_{vt}^{-1}(\delta)) \le tr(\Omega^{-1}),$$

where the first and second inequalities follow from Lemma B.1(vi) and (ix), respectively. Hence, it follows that (i) holds by the compactness of $\Theta_\delta$.

(ii) The proof follows by (5.1), (5.5), and the similar arguments as for (i).

(iii) By (B.2) and (B.3), we know that

$$\mathcal{H}_t(\delta) = \sum_{i=0}^{\infty} \mathcal{B}^i(u)\left[r(\delta) + \mathcal{A}(u)\mathcal{Y}_{t-1-i}\right]. \tag{C.8}$$

Hence, by (B.3)-(C.8), the triangle inequality, the stationarity of $Y_t$, and the compactness of $\Theta_\delta$, it follows that

$$\sup_{\delta\in\Theta_\delta} \|\mathcal{H}_t(\delta)\| \le U \sum_{i=0}^{\infty} \phi^i \left[\sup_{\delta\in\Theta_\delta} \|(r(\delta) + \mathcal{A}(u)\mathcal{Y}_{t-1-i})\|\right] \le U \sum_{i=0}^{\infty} \phi^i (U + U\|\mathcal{Y}_{t-1-i}\|).$$

Together with the Minkowski's inequality, it entails that

$$\begin{aligned} E\left[\left(\sup_{\delta\in\Theta_\delta} \|\Sigma_{vt}(\delta)\|\right)^k\right] &\le \left\{U\sum_{i=0}^{\infty}\left\{E\left[\phi^i(U+U\|\mathcal{Y}_{t-1-i}\|)\right]^k\right\}^{1/k}\right\}^k \\ &\le \left\{U\sum_{i=0}^{\infty}\phi^i\left\{1+E\|\mathcal{Y}_{t-1-i}\|^k\right\}^{1/k}\right\}^k \\ &= \left\{U\sum_{i=0}^{\infty}\phi^i\left\{1+E\|Y_t\|^k\right\}^{1/k}\right\}^k < \infty, \end{aligned}$$

i.e., (iii) holds. Similarly, we can show that (iv) and (v) hold. This completes all of the proofs. □

Proof of Lemma B.3. First, by (5.1), (5.7) and the compactness of $\Theta_\nu$, we can obtain

$$\sup_{(u,\nu)\in\Theta_u\times\Theta_\nu} \|L_T(s_0,u,\nu) - L_{T,h}(\hat{s}_v,u,\nu)\| \le \xi_1 + \xi_2, \tag{C.9}$$

where

$$\xi_1 = \frac{1}{T}\sum_{t=1}^{T}\sup_{u\in\Theta_u}\left\|\log\frac{|\Sigma_{vt}(s_0,u)|}{\left|\widehat{\Sigma}_{vt}(\hat{s}_v,u)\right|}\right\| \text{ and } \xi_2 = \frac{1}{T}\sum_{t=1}^{T}\left\|\log\frac{\left|I_n + \frac{\nu_1}{\nu_2-n-1}\Sigma_{vt}^{-1}(s_0,u)Y_t\right|}{\left|I_n + \frac{\nu_1}{\nu_2-n-1}\widehat{\Sigma}_{vt}^{-1}(\hat{s}_v,u)Y_t\right|}\right\|.$$

Next, by Lemma B.1(x), we have

$$\begin{aligned} \xi_1 &\le \frac{n}{T}\sum_{t=1}^{T}\sup_{u\in\Theta_u}\left\|\Sigma_{vt}(s_0,u) - \widehat{\Sigma}_{vt}(\hat{s}_v,u)\right\| \\ &\quad \times \left[\sup_{u\in\Theta_u}\|\Sigma_{vt}^{-1}(s_0,u)\| + \sup_{u\in\Theta_u}\|\widehat{\Sigma}_{vt}^{-1}(\hat{s}_v,u)\|\right] \\ &\le \frac{nU}{T}\sum_{t=1}^{T}\sup_{u\in\Theta_u}\left\|\Sigma_{vt}(s_0,u) - \widehat{\Sigma}_{vt}(\hat{s}_v,u)\right\|, \end{aligned} \tag{C.10}$$

where the last inequality holds by Lemma B.2(i)-(ii).

Third, we claim that there exists a constant $\phi \in (0,1)$ such that for all $t \geq 1$,

$$\sup_{u\in\Theta_u} \|\Sigma_{vt}(s_0,u) - \widehat{\Sigma}_{vt}(\hat{s}_v,u)\| \leq U\wp_1\phi^t + U\|\hat{s}_v - s_0\|, \tag{C.11}$$

where $\wp_1 > 0$ is to be specified later. By (B.1)-(B.2), it is straightforward to see that

$$\mathcal{H}_t(s_0,u) - \widehat{\mathcal{H}}_t(\hat{s}_v,u) = \mathcal{B}^t(u)(\mathcal{H}_0(s_0,u) - \widehat{\mathcal{H}}_0^*) + \sum_{i=0}^{t-1} \mathcal{B}^i(u)[r(s_0,u) - r(\hat{s}_v,u)]. \tag{C.12}$$

By (B.3), (C.12) and the compactness of $\Theta_u$, we can show that

$$\sup_{u\in\Theta_u} \|\mathcal{H}_t(s_0,u) - \widehat{\mathcal{H}}_t(\hat{s}_v,u)\| \leq U\wp_1\phi^t + U\|\hat{s}_v - s_0\|,$$

where $\wp_1 = \sup_{u\in\Theta_u} \|\mathcal{H}_0(s_0,u) - \widehat{\mathcal{H}}_0^*\|$ with $E\wp_1 < \infty$ by Lemma B.2(iii). Thus, it follows that (C.11) holds.

Now, by (C.10)-(C.11), we can obtain that

$$\xi_1 \leq \frac{U}{T}\sum_{t=1}^{T} \wp_1\phi^t + U\|\hat{s}_v - s_0\|. \tag{C.13}$$

On one hand, since $E\wp_1 < \infty$, we have $\sum_{t=1}^{\infty} \frac{\wp_1\phi^t}{t} < \infty$ a.s., which implies that

$$\frac{1}{T}\sum_{t=1}^{T} \wp_1\phi^t \xrightarrow{a.s.} 0 \quad \text{as } T \to \infty$$

by the Kronecker's lemma. On the other hand, $\hat{s}_v - s_0 \xrightarrow{a.s.} 0$ as $T \to \infty$ by the ergodic theorem. Therefore, by (C.13) it follows that $\xi_1 \xrightarrow{a.s.} 0$ as $T \to \infty$. Similarly, we can show that $\xi_2 \xrightarrow{a.s.} 0$ as $T \to \infty$, and hence the conclusion holds by (C.9). □

Proof of Lemma B.4. Let $\xi_3(\theta_v) = I_n + \frac{\nu_1}{\nu_2-n-1}\Sigma_{vt}^{-1/2}(\delta)Y_t\Sigma_{vt}^{-1/2}(\delta)$. Then, (i) holds by (5.6) and the fact that

$$\begin{aligned}
&E\left[\sup_{\theta_v\in\Theta_v} |l_{vt}(\theta_v)|\right] \\
&\leq U + UE\left[\sup_{\theta_v\in\Theta_v} \Big|\log|\Sigma_{vt}(\delta)| + \log|Y_t| + \log|\xi_3(\theta_v)|\Big|\right] \\
&\leq U + UE\Bigg[\sup_{\delta\in\Theta_\delta} \left\{tr(\Sigma_{vt}(\delta)) + tr(\Sigma_{vt}^{-1}(\delta))\right\} + tr(Y_t) + tr(Y_t^{-1}) \\
&\qquad + \sup_{\theta_v\in\Theta_v} \left\{tr(\xi_3(\theta_v)) + tr(\xi_3^{-1}(\theta_v))\right\}\Bigg]
\end{aligned}$$

$$\leq U + UE\left[\sup_{\delta\in\Theta_\delta}\left\{\|\Sigma_{vt}(\delta)\| + \|\Sigma_{vt}^{-1}(\delta)\|\right\}\right] + \left\{tr(E(Y_t)) + tr(E(Y_t^{-1}))\right\}$$
$$+ \sqrt{n}E\left[\sup_{\theta_v\in\Theta_v}\left\{\|\xi_3(\theta_v)\| + \|\xi_3^{-1}(\theta_v)\|\right\}\right] < \infty,$$

where the first inequality holds by the triangle inequality and the compactness of $\Theta_\nu$, the second inequality holds by Lemma B.1(vii), the third inequality holds by Lemma B.1(iii), and the fourth inequality holds by the fact that

$(a)$ $E\left[\sup_{\delta\in\Theta_\delta}\left\{\|\Sigma_{vt}(\delta)\| + \|\Sigma_{vt}^{-1}(\delta)\|\right\}\right] < \infty$ by Lemma B.2(i) and (iii),

$(b)$ $E\left[\sup_{\theta_v\in\Theta_v}\|\xi_3(\theta_v)\|\right] < \infty$ by the triangle inequality and Lemma B.2(i);

$(c)$ $E\left[\sup_{\theta_v\in\Theta_v}\|\xi_3^{-1}(\theta_v)\|\right] < \infty$ by Lemma B.1(vi);

$(d)$ $|tr(E(Y_t^{-1}))| \leq \sqrt{n}\|E(Y_t^{-1})\| = \dfrac{\sqrt{n}\nu_1}{\nu_2 - n - 1}\|E(\Sigma_t^{-1/2}L_t^{-1/2}R_tL_t^{-1/2}\Sigma_t^{-1/2})\|$

$\leq U\|E(L_t^{-1})\|\|ER_t\| < \infty,$ by Lemma B.1(iii), (2.5) and Lemma B.2(i).

By (i) and the uniform Law of Large Numbers for the stationary process, it follows that (ii) holds. This completes all of the proofs. □

Proof of Lemma B.5. By definition, $l_{vt}(\theta_v) = -\log[f(Y_t;\nu,\Sigma_{vt}(\delta))]$, where the density function $f(x;\nu,\Sigma_{vt}(\delta))$ is defined as in (2.2). Since the conditional density of $Y_t$ given $\mathcal{G}_{t-1}$ is $f(x;\nu_0,\Sigma_{vt}(\delta_0))$, it follows that

$$\begin{aligned}
&E\left(l_{vt}(s_0,u_0,\nu_0)\right) - E\left(l_{vt}(s_0,u,\nu)\right)\\
&\quad = E\left(\log\frac{f(Y_t;\nu,\Sigma_{vt}(s_0,u))}{f(Y_t;\nu_0,\Sigma_{vt}(s_0,u_0))}\right)\\
&\quad \leq E\left(\frac{f(Y_t;\nu,\Sigma_{vt}(s_0,u))}{f(Y_t;\nu_0,\Sigma_{vt}(s_0,u_0))} - 1\right)\\
&\quad = E\left[E\left[\frac{f(Y_t;\nu,\Sigma_{vt}(s_0,u))}{f(Y_t;\nu_0,\Sigma_{vt}(s_0,u_0))}\middle|\mathcal{G}_{t-1}\right] - 1\right]\\
&\quad = E\left[\int\frac{f(x;\nu,\Sigma_{vt}(s_0,u))}{f(x;\nu_0,\Sigma_{vt}(s_0,u_0))}f(x;\nu_0,\Sigma_{vt}(s_0,u_0))dx - 1\right]\\
&\quad = E\left[\int f(x;\nu,\Sigma_{vt}(s_0,u))dx - 1\right] = 0,
\end{aligned}$$

where the equality holds if and only if $\frac{f(Y_t;\nu,\Sigma_{vt}(s_0,u))}{f(Y_t;\nu_0,\Sigma_{vt}(s_0,u_0))} = 1$ a.s., i.e. $\Sigma_{vt}(s_0,u) = \Sigma_{vt}(s_0,u_0) =$ which is equivalent to the condition $(u,\nu) = (u_0,\nu_0)$ by Assumption 3.2 and the fact that $\Sigma_{vt}(s,u) = \Sigma_t(w,u)$. This completes the proof. □

PROOF OF LEMMA B.6. Recall that $\theta_v = (\delta', \nu')'$. For simplicity, we only prove (i) for the term $\frac{\partial^2 l_{vt}(\theta_v)}{\partial\delta_i\partial\delta_j}$, where $\delta_i$ is the $i$-th entry of $\delta$. In view of the expression of $\frac{\partial^2 l_{vt}(\theta_v)}{\partial\delta_i\partial\delta_j}$ in Appendix E, it suffices to show that the expected supremum of each term is finite. Below, we give the proof for its last term, and the proofs for the remaining terms are similar and hence omitted.

Let $\xi_4(\theta_v) = I_n + \frac{\nu_2-n-1}{\nu_1}\Sigma_{vt}^{1/2}(\delta)Y_t^{-1}\Sigma_{vt}^{1/2}(\delta)$. Then, $\varsigma_4(\theta_v)$ defined in Appendix E can be re-written as $\varsigma_4(\theta_v) = \Sigma_{vt}^{1/2}(\delta)\xi_4(\theta_v)\Sigma_{vt}^{-1/2}(\delta)$, and hence the last term of $\frac{\partial^2 l_{vt}(\theta_v)}{\partial\delta_i\partial\delta_j}$ becomes

$$tr[\Delta_{ij}(\theta_v)] := \frac{\nu_1+\nu_2}{2}tr\left[\Sigma_{vt}^{-1/2}(\delta)\xi_4^{-1}(\theta_v)\Sigma_{vt}^{-1/2}(\delta)\frac{\partial\Sigma_{vt}(\delta)}{\partial\delta_j}\Sigma_{vt}^{-1/2}(\delta)\xi_4^{-1}(\theta_v)\Sigma_{vt}^{-1/2}(\delta)\frac{\partial\Sigma_{vt}(\delta)}{\partial\delta_i}\right].$$

Note that

$$\begin{aligned}\sup_{\theta_v\in\Theta_v}\|tr[\Delta_{ij}(\theta_v)]\| &\le U\sup_{\theta_v\in\Theta_v}\left\|\Sigma_{vt}^{-1/2}(\delta)\right\|^4\left\|\xi_4^{-1}(\theta_v)\right\|^2\left\|\frac{\partial\Sigma_{vt}(\delta)}{\partial\delta_i}\right\|\left\|\frac{\partial\Sigma_{vt}(\delta)}{\partial\delta_j}\right\| \\ &\le U\left(\sup_{\delta\in\Theta_\delta}\left\|\frac{\partial\Sigma_t(\delta)}{\partial\delta_i}\right\|\right)\left(\sup_{\delta\in\Theta_\delta}\left\|\frac{\partial\Sigma_t(\delta)}{\partial\delta_j}\right\|\right), \qquad \text{(C.14)}\end{aligned}$$

where the first inequality holds by Lemma B.1(iii), the compactness of $\Theta_\nu$, and the fact that Frobenius norm is sub-multiplicative, and the second inequality holds by Lemma B.1(vi) and Lemma B.2(i). Now, by (C.14), the Holder's inequality and Lemma B.2(iv), we have

$$\begin{aligned}&E\left[\sup_{\theta_v\in\Theta_v}\|tr[\Delta_{ij}(\theta_v)]\|\right] \\ &\le U\left\{E\left[\left(\sup_{\delta\in\Theta_\delta}\left\|\frac{\partial\Sigma_t(\delta)}{\partial\delta_i}\right\|\right)^2\right]\right\}^{1/2}\left\{E\left[\left(\sup_{\delta\in\Theta_\delta}\left\|\frac{\partial\Sigma_t(\delta)}{\partial\delta_j}\right\|\right)^2\right]\right\}^{1/2} < \infty.\end{aligned}$$

Hence, we know that (i) holds. By (i) and the uniform Law of Large numbers for the stationary process, we can show that (ii) holds. This completes all of the proofs. □

PROOF OF LEMMA B.7. Let $\bar{s} = (\hat{s}_v', \hat{s}_v', \cdots, \hat{s}_v')' \in \mathcal{R}^{Mn^2\times 1}$. Then, it is straightforward to see that

$$\frac{1}{T}\sum_{t=1}^{T}\mathcal{H}_t(\delta_0) = \bar{s} - \frac{1}{T}\sum_{t=1}^{T}(\mathcal{Y}_t - \mathcal{H}_t(\delta_0)) + o_p\left(\frac{1}{\sqrt{T}}\right). \qquad \text{(C.15)}$$

By (B.2), we have

$$\frac{1}{T}\sum_{t=1}^{T}\mathcal{H}_t(\delta_0) = r(\delta_0) + \mathcal{A}(u_0)\frac{1}{T}\sum_{t=1}^{T}\mathcal{Y}_{t-1} + \mathcal{B}(u_0)\frac{1}{T}\sum_{t=1}^{T}\mathcal{H}_{t-1}(\delta_0)$$

$$= r(\delta_0) + \mathcal{A}(u_0)\frac{1}{T}\sum_{t=1}^{T}\mathcal{Y}_t + \mathcal{B}(u_0)\frac{1}{T}\sum_{t=1}^{T}\mathcal{H}_t(\delta_0) + o_p\left(\frac{1}{\sqrt{T}}\right),$$

which implies that

$$(I_{Mn^2} - \mathcal{B}(u_0))\,\frac{1}{T}\sum_{t=1}^{T}\mathcal{H}_t(\delta_0) = r(\delta_0) + \mathcal{A}(u_0)\bar{s} + o_p\left(\frac{1}{\sqrt{T}}\right). \tag{C.16}$$

Using (C.15) and (C.16), it follows that

$$\begin{aligned}(I_{Mn^2} - \mathcal{A}(u_0) - \mathcal{B}(u_0))\,\bar{s} = r(\delta_0) + (I_{Mn^2} - \mathcal{B}(u_0))\,\frac{1}{T}\sum_{t=1}^{T}(\mathcal{Y}_t - \mathcal{H}_t(\delta_0)) \\ + o_p\left(\frac{1}{\sqrt{T}}\right).\end{aligned} \tag{C.17}$$

Note that $r(\delta_0) = \mathcal{W}(I_{Mn^2} - \mathcal{A}(u_0) - \mathcal{B}(u_0))\bar{s}_0$, where $\bar{s}_0 = (s_0', s_0', \cdots, s_0')' \in \mathcal{R}^{Mn^2\times 1}$ and

$$\mathcal{W} = \begin{pmatrix} I_{n^2} & 0 & \dots & 0 \\ 0 & 0 & \ddots & \vdots \\ \vdots & \ddots & \ddots & 0 \\ 0 & \cdots & 0 & 0 \end{pmatrix}.$$

Multiplying $\mathcal{W}$ on both sides of (C.17) gives us that

$$\begin{aligned}&\mathcal{W}\left(I_{Mn^2} - \mathcal{A}(u_0) - \mathcal{B}(u_0)\right)(\bar{s} - \bar{s}_0) \\ &= \mathcal{W}(I_{Mn^2} - \mathcal{B}(u_0))\frac{1}{T}\sum_{t=1}^{T}(\mathcal{Y}_t - \mathcal{H}_t(\delta_0)) + o_p\left(\frac{1}{\sqrt{T}}\right).\end{aligned} \tag{C.18}$$

Let $\mathcal{Y}_t^* = (vec(Y_t)', vec(Y_t)', ..., vec(Y_t)')' \in \mathcal{R}^{Mn^2\times 1}$ and

$$\mathcal{H}_t^*(\delta_0) = (vec(\Sigma_{vt}(\delta_0))', vec(\Sigma_{vt}(\delta_0))', \cdots, vec(\Sigma_{vt}(\delta_0))')' \in \mathcal{R}^{Mn^2\times 1}.$$

Then, we have

$$\frac{1}{\sqrt{T}}\sum_{t=1}^{T}\mathcal{Y}_t^* = \frac{1}{\sqrt{T}}\sum_{t=1}^{T}\mathcal{Y}_t + o_p(1) \text{ and } \frac{1}{\sqrt{T}}\sum_{t=1}^{T}\mathcal{H}_t^*(\delta_0) = \frac{1}{\sqrt{T}}\sum_{t=1}^{T}\mathcal{H}_t(\delta_0) + o_p(1).$$

Combined with (C.18), it gives us that

$$\begin{aligned}&\sqrt{T}\left[\mathcal{W}\left(I_{Mn^2} - \mathcal{A}(u_0) - \mathcal{B}(u_0)\right)(\bar{s} - \bar{s}_0)\right] \\ &= \mathcal{W}(I_{Mn^2} - \mathcal{B}(u_0))\frac{1}{\sqrt{T}}\sum_{t=1}^{T}(\mathcal{Y}_t^* - \mathcal{H}_t^*(\delta_0)) + o_p(1),\end{aligned}$$

which implies that

$$\sqrt{T}\left(\hat{s}_v - s_0\right) = \Phi(u_0)\frac{1}{\sqrt{T}}\sum_{t=1}^{T} vec\left(Y_t - \Sigma_{vt}(\delta_0)\right) + o_p(1),$$

where $\Phi(u)$ is defined as in Theorem 5.2, and $vec\left(Y_t - \Sigma_{vt}(\delta_0)\right)$ is the martingale difference due to the fact that $\Sigma_{vt}(\delta_0) = \Sigma_t$ and $E(Y_t|\mathcal{G}_{t-1}) = \Sigma_t$. Hence, the conclusion holds since $\partial l_{vt}(\theta_{v0})/\partial\zeta$ is the martingale difference by Lemma B.6(i) and the standard argument for the MLE. □

Proof of Lemma B.8. In view of the expressions of $\frac{\partial l_{vt}(\theta_v)}{\partial \delta_i}$ and $\frac{\partial l_{vt}(\theta_v)}{\partial \nu_i}$ in Appendix E, we can show that

$$E\left[\left(\sup_{\theta_v\in\Theta_v}\left\|\frac{\partial l_{vt}(\theta_v)}{\partial\zeta}\right\|\right)^2\right] < \infty,$$

by using the similar argument as for Lemma B.6(i). Hence, the conclusion holds by Lemma B.7 and the martingale central limit theorem. □

Proof of Lemma B.9. Recall that $\theta_v = (\delta', \nu')'$. For simplicity, we only prove (i) with respective to $\delta_i$, where $\delta_i$ is the $i$-th entry of $\delta$. The proofs of (i) with respective to other parameters are similar and hence omitted.

Firstly, by (B.1)-(B.3) and Lemma B.2, it is not hard to show that

$$\text{(C.19)}\qquad (a)\ E\sup_{\delta\in\Theta_\delta}\left\|\Sigma_{vt}(\delta) - \widehat{\Sigma}_{vt}(\delta)\right\| = O(\phi^t);$$

$$\text{(C.20)}\qquad (b)\ E\sup_{\delta\in\Theta_\delta}\left\|\frac{\partial\Sigma_{vt}(\delta)}{\partial\delta_i} - \frac{\partial\widehat{\Sigma}_{vt}(\delta)}{\partial\delta_i}\right\| = O(t\phi^t)$$

$$\text{(C.21)}\qquad (c)\ E\sup_{\delta\in\Theta_\delta}\left\|\frac{\partial^2\Sigma_{vt}(\delta)}{\partial\delta_i\partial\delta_j} - \frac{\partial^2\widehat{\Sigma}_{vt}(\delta)}{\partial\delta_i\partial\delta_j}\right\| = O(t^2\phi^t),$$

for some constant $\phi \in (0,1)$.

Next, in view of the expression of $\frac{\partial l_{vt}(\theta_v)}{\partial \delta_i}$ in Appendix E, we can show that

$$\frac{\partial l_{vt}(\theta_v)}{\partial\delta_i} - \frac{\partial\widehat{l}_{vt}(\theta_v)}{\partial\delta_i} = tr\left[\Sigma_{vt}^{-1}(\delta)a_t(\theta_v)\frac{\partial\Sigma_{vt}(\delta)}{\partial\delta_i}\right] - tr\left[\widehat{\Sigma}_{vt}^{-1}(\delta)\widehat{a}_t(\theta_v)\frac{\partial\widehat{\Sigma}_{vt}(\delta)}{\partial\delta_i}\right],$$

where

$$a_t(\theta_v) = \frac{\nu_1}{2}I_n - \frac{\nu_1+\nu_2}{2}\xi_5^{-1}(\theta_v) \quad\text{and}\quad \widehat{a}_t(\theta_v) = \frac{\nu_1}{2}I_n - \frac{\nu_1+\nu_2}{2}\widehat{\xi}_5^{-1}(\theta_v)$$

with

$$\xi_5(\theta_v) = I_n + \frac{\nu_2 - n - 1}{\nu_1}\Sigma_{vt}(\delta)Y_t^{-1} \quad \text{and} \quad \widehat{\xi}_5(\theta_v) = I_n + \frac{\nu_2 - n - 1}{\nu_1}\widehat{\Sigma}_{vt}(\delta)Y_t^{-1}.$$

Hence, by Lemma B.1(iii) and the triangle's inequality, it follows that

$$\left\|\frac{\partial l_{vt}(\theta_v)}{\partial \delta_i} - \frac{\partial \widehat{l}_{vt}(\theta_v)}{\partial \delta_i}\right\| \leq \|b_{1t}(\theta_v)\| + \|b_{2t}(\theta_v)\| + \|b_{3t}(\theta_v)\|, \tag{C.22}$$

where $b_{1t}(\theta_v) = \left[\Sigma_{vt}^{-1}(\delta) - \widehat{\Sigma}_{vt}^{-1}(\delta)\right] a_t(\theta_v)\frac{\partial \Sigma_{vt}(\delta)}{\partial \delta_i}$, $b_{2t}(\theta_v) = \widehat{\Sigma}_{vt}^{-1}(\delta)\left[a_t(\theta_v) - \widehat{a}_t(\theta_v)\right]\frac{\partial \Sigma_{vt}(\delta)}{\partial \delta_i}$ and $b_{3t}(\theta_v) = \widehat{\Sigma}_{vt}^{-1}(\delta)\widehat{a}_t(\theta_v)\left[\frac{\partial \Sigma_{vt}(\delta)}{\partial \delta_i} - \frac{\partial \widehat{\Sigma}_{vt}(\delta)}{\partial \delta_i}\right]$.

For $b_{1t}(\theta_v)$, it is straightforward to see that

$$\begin{aligned}
\sup_{\theta_v\in\Theta_v}\|b_{1t}(\theta_v)\| &= \sup_{\theta_v\in\Theta_v}\left\|\widehat{\Sigma}_{vt}^{-1}(\delta)\left[\widehat{\Sigma}_{vt}(\delta) - \Sigma_{vt}(\delta)\right]\Sigma_{vt}^{-1}(\delta)a_t(\theta_v)\frac{\partial \Sigma_{vt}(\delta)}{\partial \delta_i}\right\| \\
&\leq U\sup_{\delta\in\Theta_\delta}\left\|\widehat{\Sigma}_{vt}^{-1}(\delta)\left[\widehat{\Sigma}_{vt}(\delta) - \Sigma_{vt}(\delta)\right]\Sigma_{vt}^{-1}(\delta)\frac{\partial \Sigma_{vt}(\delta)}{\partial \delta_i}\right\| \\
&\quad + U\sup_{\theta_v\in\Theta_v}\left\|\widehat{\Sigma}_{vt}^{-1}(\delta)\left[\widehat{\Sigma}_{vt}(\delta) - \Sigma_{vt}(\delta)\right]\Sigma_{vt}^{-1}(\delta)\xi_5^{-1}(\theta_v)\frac{\partial \Sigma_{vt}(\delta)}{\partial \delta_i}\right\| \\
&= U\sup_{\delta\in\Theta_\delta}\left\|\widehat{\Sigma}_{vt}^{-1}(\delta)\left[\widehat{\Sigma}_{vt}(\delta) - \Sigma_{vt}(\delta)\right]\Sigma_{vt}^{-1}(\delta)\frac{\partial \Sigma_{vt}(\delta)}{\partial \delta_i}\right\| \\
&\quad + U\sup_{\theta_v\in\Theta_v}\left\|\widehat{\Sigma}_{vt}^{-1}(\delta)\left[\widehat{\Sigma}_{vt}(\delta) - \Sigma_{vt}(\delta)\right]\Sigma_{vt}^{-1/2}(\delta)\xi_4^{-1}(\theta_v)\Sigma_{vt}^{-1/2}(\delta)\frac{\partial \Sigma_{vt}(\delta)}{\partial \delta_i}\right\| \\
&\leq U\left(\sup_{\delta\in\Theta_\delta}\left\|\widehat{\Sigma}_{vt}(\delta) - \Sigma_{vt}(\delta)\right\|\right)\left(\sup_{\delta\in\Theta_\delta}\left\|\frac{\partial \Sigma_{vt}(\delta)}{\partial \delta_i}\right\|\right), \qquad \text{(C.23)}
\end{aligned}$$

where the first inequality holds by the triangle's inequality, and the second inequality holds by Lemmas B.1(vi) and B.2(i)-(ii). Similarly, we can obtain that

$$\sup_{\theta_v\in\Theta_v}\|b_{2t}(\theta_v)\| \leq U\left(\sup_{\delta\in\Theta_\delta}\left\|\widehat{\Sigma}_{vt}(\delta) - \Sigma_{vt}(\delta)\right\|\right)\left(\sup_{\delta\in\Theta_\delta}\left\|\frac{\partial \Sigma_{vt}(\delta)}{\partial \delta_i}\right\|\right)\|Y_t^{-1}\|, \tag{C.24}$$

$$\sup_{\theta_v\in\Theta_v}\|b_{3t}(\theta_v)\| \leq U\sup_{\delta\in\Theta_\delta}\left\|\frac{\partial \Sigma_{vt}(\delta)}{\partial \delta_i} - \frac{\partial \widehat{\Sigma}_{vt}(\delta)}{\partial \delta_i}\right\|. \tag{C.25}$$

Note that $\|Y_t^{-1}\| \leq U tr(L_t^{-1})\|R_t\|$ and $L_t$ (or $R_t$) is independent to $\mathcal{G}_{t-1}$. By (C.22)-(C.25), it follows that

$$\begin{aligned}
E\left[\sup_{\theta_v\in\Theta_v}\left\|\frac{\partial l_{vt}(\theta_v)}{\partial \delta_i} - \frac{\partial \widehat{l}_{vt}(\theta_v)}{\partial \delta_i}\right\|\right] &\leq UE\left[\left(\sup_{\delta\in\Theta_\delta}\left\|\widehat{\Sigma}_{vt}(\delta) - \Sigma_{vt}(\delta)\right\|\right)\left(\sup_{\delta\in\Theta_\delta}\left\|\frac{\partial \Sigma_{vt}(\delta)}{\partial \delta_i}\right\|\right)\right] \\
&\quad + UE\left[\sup_{\delta\in\Theta_\delta}\left\|\frac{\partial \Sigma_{vt}(\delta)}{\partial \delta_i} - \frac{\partial \widehat{\Sigma}_{vt}(\delta)}{\partial \delta_i}\right\|\right]. \qquad \text{(C.26)}
\end{aligned}$$

Hence, by Chebyshev's inequality, for any $\varepsilon > 0$ and some $\phi \in (0,1)$,

$$
\begin{aligned}
&P\left(\sup_{\theta_v \in \Theta_v} \left\| \sqrt{T}\left(\frac{\partial L_v(\theta_v)}{\partial \delta_i} - \frac{\partial \widehat{L}_v(\theta_v)}{\partial \delta_i}\right)\right\| > \varepsilon\right) \\
&\leq \frac{1}{\varepsilon\sqrt{T}} \sum_{t=1}^{T} E\left[\sup_{\theta_v \in \Theta_v} \left\| \frac{\partial l_{vt}(\theta_v)}{\partial \delta_i} - \frac{\partial \widehat{l}_{vt}(\theta_v)}{\partial \delta_i}\right\|\right] \\
&\leq \frac{U}{\varepsilon\sqrt{T}} \sum_{t=1}^{T} (\phi^{2t} + t\phi^t) \\
&\to 0 \text{ as } T \to \infty,
\end{aligned}
$$

where the last inequality holds by (C.19), (C.20), (C.26), and Lemma B.2(iv). Hence, we know that (i) holds. Similarly, we can show that (ii) holds. This completes all of the proofs.

□

## APPENDIX D: DERIVATIVES AND STOCK LISTS

In this appendix, we list the first and second order derivatives of $l_{vt}(\theta_v)$. Let

$$
\begin{aligned}
&s_3(\nu) = \frac{\nu_1}{\nu_2 - n - 1}, \;\; s_4(\nu) = \frac{\nu_1 + \nu_2}{\nu_2 - n - 1}, \;\; s_5(\nu) = \frac{\nu_1 + \nu_2}{\nu_1}, \\
&\varsigma_0(\delta) = \Sigma_{vt}^{-1}(\delta) Y_t, \;\; \varsigma_{1i}(\delta) = \Sigma_{vt}^{-1}(\delta)\frac{\partial \Sigma_{vt}(\delta)}{\partial \delta_i}, \;\; \varsigma_{2ij}(\delta) = \Sigma_{vt}^{-1}(\delta)\frac{\partial \Sigma_{vt}(\delta)}{\partial \delta_i \partial \delta_j}, \\
&\varsigma_3(\theta_v) = I_n + s_3(\nu)\Sigma_{vt}^{-1}(\delta) Y_t, \;\; \varsigma_4(\theta_v) = I_n + s_3^{-1}(\nu) Y_t^{-1} \Sigma_{vt}(\delta).
\end{aligned}
$$

Then, by direction calculation, we have

$$
\begin{aligned}
\frac{\partial l_{vt}(\theta_v)}{\partial \nu_1} &= \frac{\partial C(\nu)}{\partial \nu_1} - \frac{1}{2}\log|s_3(\nu)\varsigma_0(\delta)| - \frac{n}{2} + \frac{1}{2}\log|\varsigma_3(\theta_v)| + \frac{s_4(\nu)}{2} tr\left[\varsigma_3^{-1}(\theta_v)\varsigma_0(\delta)\right], \\
\frac{\partial l_{vt}(\theta_v)}{\partial \nu_2} &= \frac{\partial C(\nu)}{\partial \nu_2} + \frac{n s_3(\nu)}{2} + \frac{1}{2}\log|\varsigma_3(\theta_v)| - \frac{s_3(\nu)s_4(\nu)}{2} tr\left[\varsigma_3^{-1}(\theta_v)\varsigma_0(\delta)\right], \\
\frac{\partial l_{vt}(\theta_v)}{\partial \delta_i} &= \frac{\nu_1}{2} tr[\varsigma_{1i}(\delta)] - \frac{\nu_1 + \nu_2}{2} tr[\varsigma_4^{-1}\varsigma_{1i}(\delta)],
\end{aligned}
$$

and

$$
\begin{aligned}
\frac{\partial^2 l_{vt}(\theta_v)}{\partial \nu_1^2} &= \frac{\partial C(\nu)}{\partial \nu_1^2} - \frac{n}{2\nu_1} + \frac{1}{(\nu_2 - n - 1)} tr[\varsigma_3(\theta_v)^{-1}\varsigma_0(\delta)] \\
&\quad - \frac{s_4(\nu)}{2(\nu_2 - n - 1)} tr[\varsigma_3^{-1}(\theta_v)\varsigma_0(\delta)\varsigma_3^{-1}(\theta_v)\varsigma_0(\delta)], \\
\frac{\partial^2 l_{vt}(\theta_v)}{\partial \nu_2^2} &= \frac{\partial C(\nu)}{\partial \nu_2^2} - \frac{n s_3(\nu)}{2(\nu_2 - n - 1)} + [s_3(\nu)\frac{(\nu_1 + n + 1)}{(\nu_2 - n - 1)^2}] tr[\varsigma_3(\theta_v)^{-1}\varsigma_0(\delta)] \\
&\quad - \frac{s_3^2(\nu)s_4(\nu)}{2(\nu_2 - n - 1)} tr[\varsigma_3^{-1}(\theta_v)\varsigma_0(\delta)\varsigma_3^{-1}(\theta_v)\varsigma_0(\delta)],
\end{aligned}
$$

$$\frac{\partial^2 l_{vt}(\theta_v)}{\partial\nu_1\partial\nu_2} = \frac{\partial C(\nu)}{\partial\nu_1\partial\nu_2} + \frac{n}{2(\nu_2-n-1)} + \left[\frac{s_3(\nu)}{2\nu_1} - \frac{s_3(\nu)+s_4(\nu)}{2(\nu_2-n-1)}\right] tr\left[\varsigma_3^{-1}(\theta_v)\varsigma_0(\delta)\right]$$
$$+ \frac{s_3(\nu)s_4(\nu)}{2(\nu_2-n-1)} tr\left[\varsigma_3^{-1}(\theta_v)\varsigma_0(\delta)\varsigma_3^{-1}(\theta_v)\varsigma_0(\delta)\right],$$
$$\frac{\partial^2 l_{vt}(\theta_v)}{\partial\delta_i\partial\nu_1} = \frac{1}{2}tr[\varsigma_{1i}(\delta)] - \frac{1}{2}tr[\varsigma_4^{-1}\varsigma_{1i}(\delta)] - \frac{s_5(\nu)}{2s_3(\nu)}tr[\varsigma_4^{-1}\varsigma_{1i}(\delta)\varsigma_4^{-1}\varsigma_0(\delta)^{-1}]$$
$$\frac{\partial^2 l_{vt}(\theta_v)}{\partial\delta_i\partial\nu_2} = -\frac{1}{2}tr[\varsigma_4^{-1}\varsigma_{1i}(\delta)] + \frac{s_5(\nu)}{2}tr[\varsigma_4^{-1}\varsigma_{1i}(\delta)\varsigma_4^{-1}\varsigma_0(\delta)^{-1}]$$
$$\frac{\partial^2 l_{vt}(\theta_v)}{\partial\delta_i\partial\delta_j} = \frac{\nu_1}{2}tr\left[\varsigma_{2ij}(\delta) - \varsigma_{1i}(\delta)\varsigma_{1j}(\delta)\right] - \frac{\nu_1+\nu_2}{2}tr\left[\varsigma_{2ij}(\delta)\varsigma_4^{-1}(\theta_v)\right]$$
$$+ \frac{\nu_1+\nu_2}{2}tr\left[\varsigma_4^{-1}(\theta_v)(\varsigma_{1j}(\delta)\varsigma_{1i}(\delta) + \varsigma_{1i}(\delta)\varsigma_{1j}(\delta))\right]$$
$$- \frac{\nu_1+\nu_2}{2}tr\left[\varsigma_4^{-1}(\theta_v)\varsigma_{1j}(\delta)\varsigma_4^{-1}(\theta_v)\varsigma_{1i}(\delta)\right].$$

Similarly, we can easily write down the first and second order derivatives of $l_t(\theta)$.

We now give the first and second order derivatives for $\Sigma_{vt}(\delta)$. Denote $A_{ki,lm}$ the $(l,m)$th entry of $A_{ki}$, and $B_{kj,lm}$ the $(l,m)$th entry of $B_{kj}$, $S_{lm}$ the $(l,m)$th entry of $S$, and let $J_{lm}$ be an $n\times n$ matrix zeros everywhere except for a one at the $(l,m)$th entry.

$$\frac{\partial\Sigma_{vt}(\delta)}{\partial A_{k_1i,lm}} = J_{lm}(Y_{t-i}-S)A'_{k_1i} + A_{k_1i}(Y_{t-i}-S)J'_{lm} + \sum_{j=1}^{Q}\sum_{k=1}^{K} B_{kj}\frac{\partial\Sigma_{vt-j}(\delta)}{\partial A_{k_1i,lm}}B'_{kj},$$
$$\frac{\partial\Sigma_{vt}(\delta)}{\partial B_{k_1j_1,lm}} = J_{lm}(\Sigma_{t-j_1}-S)B'_{k_1j_1} + B_{k_1j_1}(\Sigma_{t-j_1}-S)J'_{lm}$$
$$+ \sum_{j=1}^{Q}\sum_{k=1}^{K} B_{kj}\frac{\partial\Sigma_{vt-j}(\delta)}{\partial B_{k_1j_1,lm}}B'_{kj},$$
$$\frac{\partial\Sigma_{vt}(\delta)}{\partial S_{lm}} = J_{lm} - \sum_{i=1}^{P}\sum_{k=1}^{K} A_{ki}J_{lm}A'_{ki} - \sum_{j=1}^{Q}\sum_{k=1}^{K} B_{kj}[J_{lm} - \frac{\partial\Sigma_{vt-j}(\delta)}{\partial S_{lm}}]B'_{kj},$$
$$\frac{\partial^2\Sigma_{vt}(\delta)}{\partial A_{k_1i,lm}\partial A_{k_1i,qr}} = J_{lm}(Y_{t-i}-S)J'_{qr} + J_{qr}(Y_{t-i}-S)J'_{lm}$$
$$+ \sum_{j=1}^{Q}\sum_{k=1}^{K} B_{kj}\frac{\partial^2\Sigma_{vt-j}(\delta)}{\partial A_{k_1i,lm}\partial A_{k_1i,qr}}B'_{kj},$$
$$\frac{\partial\Sigma_{vt}(\delta)}{\partial B_{k_1j_1,lm}\partial B_{k_2j_2,qr}} = \mathbf{1}_{\{k_1=k_2,j_1=j_2\}}\left[J_{lm}(\Sigma_{t-j_1}-S)J'_{qr} + J_{qr}(\Sigma_{t-j_1}-S)J'_{lm}\right]$$
$$+ J_{lm}\frac{\partial\Sigma_{t-j1}}{\partial B_{k_2j_2,qr}}B'_{k_1,j_1} + B_{k_1,j_1}\frac{\partial\Sigma_{t-j1}}{\partial B_{k_2j_2,qr}}J'_{lm}$$
$$+ J_{qr}\frac{\partial\Sigma_{t-j2}}{\partial B_{k_1j_1,lm}}B'_{k_2,j_2} + B_{k_2,j_2}\frac{\partial\Sigma_{t-j2}}{\partial B_{k_1j_1,lm}}J'_{qr}$$
$$+ \sum_{j=1}^{Q}\sum_{k=1}^{K} B_{kj}\frac{\partial\Sigma_{vt-j}(\delta)}{\partial B_{k_1j_1,lm}B_{k_2j_2,qr}}B'_{kj},$$

$$
\begin{aligned}
\frac{\partial \Sigma_{vt}(\delta)}{\partial A_{k_1 i,lm}\partial B_{k_2 j_1,qr}} =& J_{qr}\frac{\partial \Sigma_{vt-j_1}(\delta)}{\partial A_{k_1 i,lm}}B'_{k_1 j_1} + B_{k_1 j_1}\frac{\partial \Sigma_{vt-j_1}(\delta)}{\partial A_{k_1 i,lm}}J'_{qr} \\
&+ \sum_{j=1}^{Q}\sum_{k=1}^{K} B_{kj}\frac{\partial \Sigma_{vt-j}(\delta)}{\partial A_{k_1 i,lm}\partial B_{k_2 j_1,qr}}B'_{kj}, \\
\frac{\partial \Sigma_{vt}(\delta)}{\partial A_{k_1 i,lm}\partial S_{qr}} =& - J_{lm}J_{qr}A'_{k_1 i} - A_{k_1 i}J_{qr}J'_{lm} + \sum_{j=1}^{Q}\sum_{k=1}^{K} B_{kj}\frac{\partial \Sigma_{vt-j}(\delta)}{\partial A_{k_1 i,lm}\partial S_{qr}}B'_{kj}, \\
\frac{\partial \Sigma_{vt}(\delta)}{\partial B_{k_1 j,lm}\partial S_{qr}} =& J_{lm}\Big[\frac{\partial \Sigma_{vt-j_1}}{\partial S_{qr}} - J_{qr}\Big]B'_{k_1 j_1} + B_{k_1 j_1}\Big[\frac{\partial \Sigma_{vt-j_1}}{\partial S_{qr}} - J_{qr}\Big]J'_{lm} \\
&+ \sum_{j=1}^{Q}\sum_{k=1}^{K} B_{kj}\frac{\partial \Sigma_{vt-j}(\delta)}{\partial B_{k_1 j_1,lm}\partial S_{qr}}B'_{kj}.
\end{aligned}
$$

$$
\begin{aligned}
&\frac{\partial \mathfrak{Z}_{vt}(\delta)}{\partial \delta_i} \\
=&\frac{\partial vec(\Sigma_{vt}^{-1/2}(\delta)Y_t\Sigma_{vt}^{-1/2}(\delta))}{\partial \delta_i} \\
=& - (\Sigma_{vt}^{-1/2}(\delta)Y_t\Sigma_{vt}^{-1/2}(\delta) \otimes \Sigma_{vt}^{-1/2}(\delta))\frac{vec(\partial \Sigma_{vt}^{1/2}(\delta))}{\partial \delta_i} \\
&- (\Sigma_{vt}^{-1/2}(\delta) \otimes \Sigma_{vt}^{-1/2}(\delta)Y_t\Sigma_{vt}^{-1/2}(\delta))\frac{vec(\partial \Sigma_{vt}^{1/2}(\delta))}{\partial \delta_i} \\
=& - (\Sigma_{vt}^{-1/2}(\delta)Y_t\Sigma_{vt}^{-1/2}(\delta) \otimes \Sigma_{vt}^{-1/2}(\delta))(\Sigma_{vt}^{1/2}(\delta) \otimes I_n + I_n \otimes \Sigma_{vt}^{1/2}(\delta))^{-1}\frac{vec(\partial \Sigma_{vt}(\delta))}{\partial \delta_i} \\
&- (\Sigma_{vt}^{-1/2}(\delta) \otimes \Sigma_{vt}^{-1/2}(\delta)Y_t\Sigma_{vt}^{-1/2}(\delta))(\Sigma_{vt}^{1/2}(\delta) \otimes I_n + I_n \otimes \Sigma_{vt}^{1/2}(\delta))^{-1}\frac{vec(\partial \Sigma_{vt}(\delta))}{\partial \delta_i}
\end{aligned}
$$

## REFERENCES


[1] Boussama, F., Fuchs, F. and Stelzer, R. (2011). Stationarity and geometric ergodicity of BEKK multivariate GARCH models. *Stochastic Processes and their Applications* **121**, 2331–2360.

[2] Newey, W. K. and McFadden, D. (1994). Large sample estimation and hypothesis testing. *Handbook of Econometrics* **4**, 2111–2245.

[3] Pedersen, R.S. and Rahbek, A. (2014). Multivariate variance targeting in the BEKK–GARCH model. *Econometrics Journal* **17**, 24–55.



University of Florida
Department of Statistics
Florida, U.S.A.
E-mail: zhou.j@ufl.edu

Center for Statistical Science
and Department of Industrial Engineering
Tsinghua University
Beijing 100084, China
E-mail: jfy16@mails.tsinghua.edu.cn

The University of Hong Kong
Department of Statistics & Actuarial Science
Hong Kong
E-mail: mazhuke@hku.hk

The Education University of Hong Kong
Department of Mathematics and Information Technology
Hong Kong
E-mail: waikeungli@eduhk.hk
